# Supplementary material for: Kirchhoff-Love shell theory based on tangential differential calculus
Source: arXiv:1805.11978 source file (2018-10-10)
Supplement: Supplementary file 1 [file CodeAppendix_Classic.pdf]

```
function [ElemMat, ElemRhs] = GetElementMatrixCurviLinear(ShapeFctsRef, ipRef, ...
   Parameters, CoordRealElem)

   % Compute element stiffness matrix based on curvilinear coordinates
   % following Kiendl et al., Comp. Methods Appl. Mech. Engrg., 198, 39023914, 2009.
   %
   % Input variables:
   % ShapeFctsRef is a data structure storing reference shape functions and
   %  derivatives as members. Each member is an (n x m)-matrix of n shape
   %  functions evaluated at m integration points. Existing members:
   %  -ShapeFctsRef.NodeNum: Number n of shape functions in this element/knot span.
   %  -ShapeFctsRef.f: shape functions (e.g., NURBS or classical FE functions).
   %  -ShapeFctsRef.fx, .fy: 1st derivatives of the shape functions.
   %  -ShapeFctsRef.fxx, .fxy, .fyy: 2nd derivatives of the shape functions.
   % ipRef stores the integration points and weights in the reference element:
   %  -ipRef.nQ: Number of integration points.
   %  -ipRef.xx, ipRef.yy: Coordinates of integration points.
   %  -ipRef.ww: Integration weights.
   % Parameters stores material parameters.
   % CoordRealElem stores the 3D coordinates of the real curved element.
   %  -CoordRealElem.xx, .yy, .zz: (x,y,z)-coordinates
   %
   % Output variables:
   % ElemMat: Element matrix.
   % ElemRhs: Element right hand side.

   % Initialization.
   nn = ShapeFctsRef.NodeNum;
   ElemMat = zeros(3*nn, 3*nn); % Size of element matrix.
   ElemRhs = zeros(3*nn, 1); % Size of element right hand side.

   % Integration points in real curved shell element.
   ipReal.nQ = ipRef.nQ;
   ipReal.xx = ShapeFctsRef.f' * CoordRealElem.xx;
   ipReal.yy = ShapeFctsRef.f' * CoordRealElem.yy;
   ipReal.zz = ShapeFctsRef.f' * CoordRealElem.zz;

   % Loading in x-, y-, z-direction evaluated at integration points.
   [fx, fy, fz] = EvaluateLoad(ipReal.xx, ipReal.yy, ipReal.zz);

   % Material parameters.
   EE = Parameters.EE;
   nu = Parameters.nu;
   tt = Parameters.tt;
   Dmemb = EE*tt/(1-nu^2);
   Dbend = EE*tt^3/12/(1-nu^2);

   % Loop over integration points.
   for i = 1 : ipRef.nQ

   % Reference shape functions at current integration point.
   N = ShapeFctsRef.f(:, i);
   Nr = ShapeFctsRef.fx(:, i); Ns = ShapeFctsRef.fy(:, i);
   Nrr = ShapeFctsRef.fxx(:, i); Nrs = ShapeFctsRef.fxy(:, i); Nss = ShapeFctsRef.fyy(:, i);

   % Get covariant basis.
   A1Cov = [Nr'*CoordRealElem.xx; Nr'*CoordRealElem.yy; Nr'*CoordRealElem.zz];
   A2Cov = [Ns'*CoordRealElem.xx; Ns'*CoordRealElem.yy; Ns'*CoordRealElem.zz];

   % Get partial derivatives of covariant basis vectors.
   A1Cov_1 = [Nrr'*CoordRealElem.xx; Nrr'*CoordRealElem.yy; Nrr'*CoordRealElem.zz];
   A1Cov_2 = [Nrs'*CoordRealElem.xx; Nrs'*CoordRealElem.yy; Nrs'*CoordRealElem.zz]; %=A2Cov_1
   A2Cov_2 = [Nss'*CoordRealElem.xx; Nss'*CoordRealElem.yy; Nss'*CoordRealElem.zz];

   % Normal vector.
   A3tilde = cross(A1Cov, A2Cov);
   A3bar = norm(A3tilde);
   A3 = A3tilde / A3bar;
```

```
    % Get covariant metric tensor.
    A11Cov = dot(A1Cov, A1Cov); A12Cov = dot(A1Cov, A2Cov); A22Cov = dot(A2Cov, A2Cov);
    AACov = [A11Cov A12Cov; A12Cov A22Cov];

    % Get contravariant metric tensor.
    AACont = inv(AACov);
    A11Cont = AACont(1,1);
    A12Cont = AACont(1,2);
    A22Cont = AACont(2,2);

    % Evaluate constitutive matrix.
    c1111 = A11Cont^2;
    c1122 = nu * A11Cont * A22Cont + (1-nu) * A12Cont^2;
    c1112 = A11Cont * A12Cont;
    c2222 = A22Cont^2;
    c2212 = A12Cont * A22Cont;
    c1212 = 1/2 * ((1+nu) * A12Cont^2 + (1-nu) * A11Cont * A22Cont);

    H = [c1111 c1122 c1112;
    c1122 c2222 c2212;
    c1112 c2212 c1212];

    Hmemb = Dmemb * H;
    Hbend = Dbend * H;

    % Compute membrane stiffness.
    m11 = [Nr' * A1Cov(1), Nr' * A1Cov(2), Nr' * A1Cov(3)];
    m22 = [Ns' * A2Cov(1), Ns' * A2Cov(2), Ns' * A2Cov(3)];
    m12 = [...
        0.5 * (Nr' * A2Cov(1) + Ns' * A1Cov(1)), ...
        0.5 * (Nr' * A2Cov(2) + Ns' * A1Cov(2)), ...
        0.5 * (Nr' * A2Cov(3) + Ns' * A1Cov(3))];
    M = [m11; m22; 2*m12];
    KKmemb = M' * Hmemb * M;

    % Compute bending stiffness.
    b11Q = Nrr' - 1/A3bar*(dot(cross(A2Cov, A3), A1Cov_1)*Nr' ...
        + dot(cross(A3, A1Cov), A1Cov_1)*Ns');
    b22Q = Nss' - 1/A3bar*(dot(cross(A2Cov, A3), A2Cov_2)*Nr' ...
        + dot(cross(A3, A1Cov), A2Cov_2)*Ns');
    b12Q = Nrs' - 1/A3bar*(dot(cross(A2Cov, A3), A1Cov_2)*Nr' ...
        + dot(cross(A3, A1Cov), A1Cov_2)*Ns');
    b11 = [A3(1) * b11Q, A3(2) * b11Q, A3(3) * b11Q];
    b22 = [A3(1) * b22Q, A3(2) * b22Q, A3(3) * b22Q];
    b12 = [A3(1) * b12Q, A3(2) * b12Q, A3(3) * b12Q];
    B = [b11; b22; 2*b12];
    KKbend =  B' * Hbend * B;

    % Right hand side, contribution at integration point.
    Rhs = [N*fx(i); N*fy(i); N*fz(i)];

    % Add contribution at integration point to element matrix and rhs.
    ElemMat = ElemMat + ipRef.ww(i)*A3bar * (KKmemb + KKbend);
    ElemRhs = ElemRhs + ipRef.ww(i)*A3bar * Rhs;

end

function [fx, fy, fz] = EvaluateLoad(xx, yy, zz)

    nn = length(xx);
    fx = zeros(nn, 1);
    fy = zeros(nn, 1);
    fz = zeros(nn, 1);

end
```
