# Supplementary material for: Kirchhoff-Love shell theory based on tangential differential calculus
Source: arXiv:1805.11978 source file (2018-10-10)
Supplement: Supplementary file 2 [file CodeAppendix_TDC.pdf]

```
function [ElemMat, ElemRhs] = GetElementContributionShell(...
   ShapeFcts, ipReal, Parameters, NormalVectors)

   % Compute element stiffness matrix.
   %
   % Input variables:
   % ShapeFcts is a data structure storing shape functions and their surface
   % derivatives as members. Each member is an (n x m)-matrix of n shape
   % functions evaluated at m integration points. Existing members:
   % -ShapeFcts.NodeNum: Number n of shape functions in this element/know span.
   % -ShapeFcts.f: shape functions (e.g., NURBS or classical FE functions).
   % -ShapeFcts.fx, .fy, .fz: Surface gradient applied to each shape function.
   % -ShapeFcts.fxx, .fyy, .fzz, .fxy, .fxz, .fyz: *Covariant* 2nd derivatives
   % of the shape functions.
   % ipReal stores the integration points and weights in members:
   % -ipReal.nQ: Number of integration points.
   % -ipReal.xx, ipReal.yy, ipReal.zz: Coordinates of integration points.
   % -ipReal.ww: Integration weights.
   % Parameters stores material parameters.
   % NormalVectors is a matrix with 3 columns storing the normal vector
   % components at each integration point.
   %
   % Output variables:
   % ElemMat: Element matrix.
   % ElemRhs: Element right hand side.

   nn = ShapeFcts.NodeNum;
   ElemMat = zeros(3*nn, 3*nn); % Size of element matrix.
   ElemRhs = zeros(3*nn, 1); % Size of element right hand side.

   % Material parameters.
   DD = Parameters.DD;
   nu = Parameters.nu;
   mu = Parameters.mu;
   lambda = Parameters.lambda;
   tt = Parameters.tt;

   % Loading in x-, y-, z-direction evaluated at integration points.
   [fx, fy, fz] = EvaluateLoad(ipReal.xx, ipReal.yy, ipReal.zz);

   % Loop over integration points.
   for i = 1 : ipReal.nQ

   % Read out shape functions and derivatives at current integration point.
   N = ShapeFcts.f(:, i);
   Nx = ShapeFcts.fx(:, i); Ny = ShapeFcts.fy(:, i); Nz = ShapeFcts.fz(:, i);
   Nxx = ShapeFcts.fxx(:, i); Nyy = ShapeFcts.fyy(:, i); Nzz = ShapeFcts.fzz(:, i);
   Nxy = ShapeFcts.fxy(:, i); Nxz = ShapeFcts.fxz(:, i); Nyz = ShapeFcts.fyz(:, i);

   % Define projectors, (3x3)-matrices:
   Q = NormalVectors(i, :)' * NormalVectors(i, :);
   P = eye(3,3) - Q;

   % Membrane stiffness, contribution at integration point.
   Mat11 = (lambda+2*mu) * Nx*Nx' + mu * Ny*Ny' + mu * Nz*Nz';
   Mat12 = lambda * Nx*Ny' + mu  * Ny*Nx';
   Mat13 = lambda * Nx*Nz' + mu  * Nz*Nx';

   Mat21 = lambda * Ny*Nx' + mu  * Nx*Ny';
   Mat22 = (lambda+2*mu) * Ny*Ny' + mu * Nx*Nx' + mu * Nz*Nz';
   Mat23 = lambda * Ny*Nz' + mu  * Nz*Ny';

   Mat31 = lambda * Nz*Nx' + mu  * Nx*Nz';
   Mat32 = lambda * Nz*Ny' + mu  * Ny*Nz';
   Mat33 = (lambda+2*mu) * Nz*Nz' + mu * Nx*Nx' + mu * Ny*Ny';
```

```
   KKmemb11 = P(1,1)*Mat11 + P(1,2)*Mat21 + P(1,3)*Mat31;
   KKmemb12 = P(1,1)*Mat12 + P(1,2)*Mat22 + P(1,3)*Mat32;
   KKmemb13 = P(1,1)*Mat13 + P(1,2)*Mat23 + P(1,3)*Mat33;

   KKmemb21 = P(2,1)*Mat11 + P(2,2)*Mat21 + P(2,3)*Mat31;
   KKmemb22 = P(2,1)*Mat12 + P(2,2)*Mat22 + P(2,3)*Mat32;
   KKmemb23 = P(2,1)*Mat13 + P(2,2)*Mat23 + P(2,3)*Mat33;

   KKmemb31 = P(3,1)*Mat11 + P(3,2)*Mat21 + P(3,3)*Mat31;
   KKmemb32 = P(3,1)*Mat12 + P(3,2)*Mat22 + P(3,3)*Mat32;
   KKmemb33 = P(3,1)*Mat13 + P(3,2)*Mat23 + P(3,3)*Mat33;

   KKmemb = tt * [...
       KKmemb11 KKmemb12 KKmemb13;
       KKmemb21 KKmemb22 KKmemb23;
       KKmemb31 KKmemb32 KKmemb33];

   % Bending stiffness, contribution at integration point.
   % ...covariant Hesse contraction (with covariant derivatives)
   K1 = Nxx*Nxx' + Nyy*Nyy' + Nzz*Nzz' + 2*(Nxy*Nxy' + Nxz*Nxz' + Nyz*Nyz');
   % ...Bi-Laplace-Beltrami
   K2 = (Nxx+Nyy+Nzz) * (Nxx+Nyy+Nzz)';
   MatWW = (1-nu) * K1 + nu * K2;

   KKbend = DD * [...
       MatWW*Q(1,1) MatWW*Q(1,2) MatWW*Q(1,3);
       MatWW*Q(2,1) MatWW*Q(2,2) MatWW*Q(2,3);
       MatWW*Q(3,1) MatWW*Q(3,2) MatWW*Q(3,3)];

   % Right hand side, contribution at integration point.
   Rhs1 = N * fx(i);
   Rhs2 = N * fy(i);
   Rhs3 = N * fz(i);
   Rhs = [Rhs1; Rhs2; Rhs3];

   % Add contribution at integration point to element matrix and rhs.
   ElemMat = ElemMat + ipReal.ww(i) * (KKmemb + KKbend);
   ElemRhs = ElemRhs + ipReal.ww(i) * Rhs;

end

function [fx, fy, fz] = EvaluateLoad(xx, yy, zz)

   nn = length(xx);
   fx = zeros(nn, 1);
   fy = zeros(nn, 1);
   fz = zeros(nn, 1);

end
```
